# Supplementary material for: Temporal Volatility Surface Projection: Parametric Surface Projection Method for Derivatives Portfolio Risk Management
Source: arXiv:2311.14985 source file (2023-11-25)
Supplement: Supplementary file 1 [file appendix.tex]

\section{Appendix: Critique by HRA}\label{sec:appendix}

Your paper seems comprehensive and very nicely written. I can't hide that I am quite impressed and pleasantly surprised with your writing style. You've also nicely summarized the existing literature and pointed out gaps your research aims to fill. Despite its merits, several aspects can be improved to make the paper more compelling and academically rigorous.

\subsection{Critique of the Introduction Section}

\begin{enumerate}

\item \textbf{Clarity and Structure:}
The introduction is overall well-structured but could benefit from clearer delineation between the research gaps, objectives, and contributions. It may be beneficial to state the main research questions and hypotheses explicitly. People have lots of respect for this in academia, and the referees of your work are from this side of the game!

\textbf{Suggestion:}
Consider adding a paragraph stating the main research questions, objectives, and hypotheses. This will help the reader immediately understand the core focus of the paper.

\textbf{Answer:}
The introduction has been refined to enhance clarity, including adding a figure depicting the hierarchy of studies and their relevance to our research. Furthermore, in the third paragraph on the third page, we have elucidated our primary objective to the audience. This revision aims to provide a more coherent and scholarly content presentation.

\item \textbf{Justification for Study:}
While the paper implies that the Black-Scholes model is insufficient under specific market conditions, explaining why understanding these shortcomings is crucial for academia and industry would be beneficial.

\textbf{Suggestion:}
Explicitly state the implications of your study for the field of quantitative finance and perhaps even for policy-making or industry best practices. This is specifically important since you mentioned something about regulators if I remember correctly. 

\textbf{Answer:}
In the third paragraph on the third page, we have elucidated our primary objective to the audience. This revision aims to provide a more coherent and scholarly content presentation. In addition, the first and second paragraphs on the second page provide a detailed explanation of why the conventional Black-Scholes-Merton (BSM) model falls short in addressing specific market conditions.

\item \textbf{Literature Review:}
You've included many references, which is good, but the current format makes it hard to distinguish between seminal works and more incremental contributions.

\textbf{Suggestion:}
Structure the literature review in a way that helps the reader understand the historical development of risk assessment models, and where your work fits in this timeline. In addition, point out clearly which reference has made a breakthrough advancement. 

\textbf{Answer:}
The introduction has been refined to enhance clarity, including adding a figure depicting the hierarchy of studies and their relevance to our research.

\item \textbf{Figures:}
Figures are referenced before they appear, which might confuse the reader. Move the figures closer to their first mention in the text to improve flow and comprehension.

\textbf{Answer:}
Done!

\item \textbf{Grammar and Stylistic Issues:}
Some sentences are quite long and could be broken down for clarity.

\textbf{Example:}
Original: "Despite its inherent assumption of constant volatility, the Black-Scholes model retains its significance in diverse research endeavors due to its simplicity."
Suggestion: "Despite its simplistic assumption, the Black-Scholes model remains a benchmark due to its simplicity." There were numerous other examples. Write simply, and make people happy!

\item \textbf{Future Work:}
The introduction might benefit from a hint at potential future work. Mention areas this study does not cover but could be of interest for future research. I spoke with Dr. Zamani at some point about the currencies, which are highly related. Another example would be bitcoins, but I do not know much about them myself. 

\textbf{Answer:}
The final paragraphs are dedicated to outlining future directions for research and development.

\end{enumerate}

\subsection{Critique for Methodology}

Overall, the methodology section is well-written and organized. Let me be a bit picky:

\begin{enumerate}
\item \textbf{Clarification Needed:} The methodology introduces two fundamentally different phenomena, interest rate curves, and implied volatility surfaces, but it does not entirely clarify how the paper will reconcile or connect these two or how they are related. As promised in the introduction, make sure to clarify how they will be integrated into the single analysis.

\textbf{Answer:}
We have provided a detailed explanation of this section, complemented by including Figure 5.

\item \textbf{Terminology:} The paper often uses "sample points" when discussing interest rates and volatility, which could confuse the reader. Specifying what these sample points represent in each context would be better.

\textbf{Answer:}
Done!

\item \textbf{Data Source:} While the paper mentions that the swap rate data is obtained from FRED, it does not specify the source for the implied volatility data. This should be clarified for completeness.

\textbf{Answer:}
It is referenced in the third footnote in the introduction section.

\item \textbf{Reference to Figures:} It would be more informative to discuss the key points and findings from Figures \ref{fig:Yield Curve (2000-07-18)} and \ref{fig:Yield Curve-IVS}, rather than simply stating they exist. I know that you have provided details in the captions but make sure you also include some remarks in the text. 

\textbf{Answer:}
It is elaborated upon in the description of the first segment of Figure 5.

\end{enumerate}

\subsection{Critique for Volatility surface based on (non)parametric representations}
\begin{enumerate}
\item \textbf{Specificity:} The paper would benefit from specifying which (if any) parametric or non-parametric models were applied in this study and why.

\textbf{Answer:}
In this section, we provide an elaborate explanation of the selected method, the cubic B-spline method, which serves as our baseline for this study.

\item \textbf{Mathematical Formalism:} The section could be enhanced by introducing mathematical equations representing parametric and non-parametric models. 

\textbf{Answer:}
We have thoroughly covered the mathematical formulas associated with well-known parametric and non-parametric methods.

\item \textbf{Arbitrage:} While the text mentions the importance of no-arbitrage conditions, it could elaborate on how these are tested or assured in the applied methods. Based on personal experience I know that these are especially of interest in capital markets. 

\textbf{Answer:}
We have presented an overview of arbitrage tests and their implications on representation models like SVI.

\item \textbf{Criteria for Data Filtering:} While you mentioned some specific criteria applied for data inclusion/exclusion, these could be better justified. Why were these specific criteria chosen? What are the alternatives? What are the pros and cons?

\textbf{Answer:}
We have provided a comprehensive explanation of the rationale behind data filtering methods.

\end{enumerate}

\subsection{Critique for S\&P 500 volatility surface vs. the VIX}
\begin{enumerate}
\item \textbf{Explicit Comparisons:} The paper could benefit from an explicit comparison between the S\&P 500 volatility surface and the VIX rather than just stating their respective features. I still do not know what is the difference, to be completely honest and clear on this. I assume many readers do not know, as well.

\textbf{Answer:}
We have clarified the distinctions between the VIX and the Implied Volatility Surface (IVS) of the S\&P 500, as well as their respective impacts on portfolio evaluation.

\item \textbf{Methodology Gap:} While the paper discusses the VIX and S\&P 500 volatility, it doesn't explain how these will be used in the subsequent analysis or model.

\textbf{Answer:}
We have now elucidated how these variables will be utilized in the forthcoming analysis or model.

\item \textbf{Clarification:} "Localized market movements" and "broader market trends" are somewhat vague and could be better defined.

\textbf{Answer:}
Done!

\end{enumerate}

\subsection{Critique for Risk measurement}
\begin{enumerate}
\item \textbf{Model Assumptions:} Value-at-risk models come with their own assumptions and limitations. An in-depth discussion regarding these could make the section more comprehensive.

\textbf{Answer:}
Additional paragraphs have been included to discuss the limitations of the VaR measure and how alternative measures like Expected Shortfall (ES) can address these limitations.

\item \textbf{VaR Equation:} In equation \eqref{VaR_def}, a detailed explanation of the terms used would benefit the reader's understanding.

\textbf{Answer:}
A comprehensive explanation has been included, offering additional insights into the estimation of the cumulative distribution of portfolio changes using various methods, including Monte Carlo simulation, historical simulation, and parametric approaches.

\item \textbf{Other Risk Measures:} VaR is a single risk measure with limitations. Have you considered using or comparing it with other measures like CVaR (Conditional Value at Risk), Entropic VaR, etc? Or maybe you have but still have not put it in the document.

\textbf{Answer:}
As stated in the initial footnote of the paper's introduction, our primary focus is on estimating the empirical distribution of portfolio value changes. Consequently, other risk measures can be readily calculated. In this study, however, our main emphasis aligns with the calculation of the VaR risk measure, which is consistent with the approach taken in \cite{zamani2022pathwise}.

\item \textbf{Monte Carlo and Historical Simulation:} It is mentioned that these methods will be integrated for VaR estimation. However, the methodology for this integration is not described. This is a critical part of your methodology and should be explained in detail.

\textbf{Answer:}
As mentioned in the concluding paragraph of this section, Section \ref{sec: PSP} is dedicated to providing a detailed explanation of this topic.

\end{enumerate}

\subsection{Parametric Surface Projection (PSP) PnL calculation}

The equations are well-defined, and the visual elements aid in comprehension. However, there are areas for improvement.

\textbf{Specific Issues}
\begin{enumerate}
    \item \textbf{Time-to-Maturity and Interest Rates}: The paper assumes that time-to-maturity and interest rates are deterministic or constant for one-day projections. While this might be reasonable for a one-day projection, justifying or providing references for these assumptions is crucial.    

    \textbf{Answer:}
    As stated in the opening sentence of the second paragraph, time-to-maturity is indeed deterministic, as the time-to-maturity for the next day will consistently be one level lower than its current value. In the context of interest rates, we have also incorporated detailed explanations elucidating why we can safely overlook its short-term fluctuations.
    
    \item \textbf{Expected Volatility}: Although the paper discusses the challenges with expected volatility and underlying asset price, it would benefit from mathematical definitions or quantifiable measures for these complexities.    

    \textbf{Answer:}
    We have explored the mathematical foundations that underlie stock price movements and their relationship with volatility fluctuations. This analysis has provided the basis for integrating these elements into a unified framework for predicting next-day prices.
    
    \item \textbf{Historical Simulation (HS)}: The methodology around the HS is discussed, but there are no details about the size of the historical data set or any justifications or citations regarding why HS is an appropriate method for capturing volatility dynamics. By the way, have you done any data augmentation for HS?

    \textbf{Answer:}
    Additional clarifications have been included for the HS component, and it's important to note that there is no data augmentation applied in this segment.
    
    \item \textbf{Monte Carlo (MC) Simulation}: The paper mentions $n$ samples from historical records but does not specify the value of $n$. Also, how do you choose the "most appropriate distribution"? Could you justify the choice of the double gamma distribution, particularly why the other candidates were rejected? Maybe you can use KS distance or some similar measure to make reasonable justifications.

    \textbf{Answer:}
    Table 1 has been excluded from the analysis due to its contradiction with the normality assumption of returns within the BSM model. Nonetheless, we recommend exploring alternative methods for modeling the underlying distribution instead of solely relying on the Gaussian process.
    
    \item \textbf{Empirical Distribution}: While Equation \eqref{eq:next-vol-agg} attempts to summarize the empirical distribution of next-day volatility, the weighting scheme ($w_i$) is not well-defined. Why was uniform weighting chosen?

    \textbf{Answer:}
    The weighting procedure is further elucidated with the introduction of various weighting schemes. Additionally, I have provided a rationale for the potential suitability of uniform weighting in this particular case.
    
    \item \textbf{Table 1 and Statistical Tests}: The paper could benefit from providing more context or interpretation for the statistical metrics displayed in Table 1. 

    \textbf{Answer:}
    Table 1 has been excluded from the analysis due to its contradiction with the normality assumption of returns within the BSM model. Nonetheless, we recommend exploring alternative methods for modeling the underlying distribution instead of solely relying on the Gaussian process.
    
    \item \textbf{Computational Complexity}: There is no mention of the computational complexity of this methodology, which could be crucial for practical implementations. Make sure you provide specifications of your machine, including number of cores and etc.

    \textbf{Answer:}
    This aspect is further elaborated upon in the subsequent section, which is dedicated to empirical results.
    
    \item \textbf{Validation and Robustness}: The paper lacks a discussion about how this methodology might be validated or its robustness tested.

    \textbf{Answer:}
    This aspect is further elaborated upon in the subsequent section, which is dedicated to empirical results.
\end{enumerate}
